# Supplementary material for: HiT-SR: Hierarchical Transformer for Efficient Image Super-Resolution
Source: arXiv:2407.05878 source file (2024-07-08)
Supplement: Supplementary file 1 [file fig-qualires-m109.tex]

% %% for supplementary materials ------------
\begin{figure*}[ht]
\tiny
\centering
\scalebox{0.92}{
\begin{tabular}{cccc}
% % one row ----------------------
\hspace{-0.2cm}
\begin{adjustbox}{valign=t}
\begin{tabular}{c}
\includegraphics[width=0.265\textwidth]{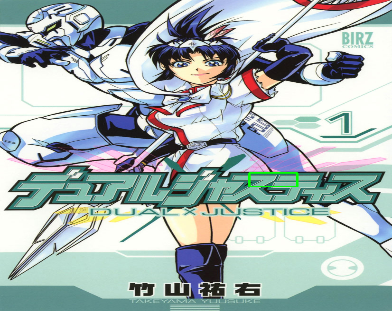}
\\
DualJustice 
\end{tabular}
\end{adjustbox}
\hspace{-0.23cm}
\begin{adjustbox}{valign=t}
\begin{tabular}{ccccc}
\includegraphics[width=0.186\textwidth]{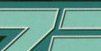} \hspace{-1.5mm} &
\includegraphics[width=0.186\textwidth]{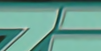} \hspace{-1.5mm} &
\includegraphics[width=0.186\textwidth]{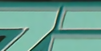} \hspace{-1.5mm} &
\includegraphics[width=0.186\textwidth]{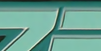} \hspace{-1.5mm} 
\\
HR \hspace{-1.5mm} &
IMDN~\cite{hui2019imdn} \hspace{-1.5mm} &
SwinIR-Light~\cite{liang2021swinir} \hspace{-1.5mm} &
SRFormer-Light~\cite{Zhou_2023srformer} \hspace{-1.5mm} 
\\
\includegraphics[width=0.186\textwidth]{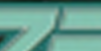} \hspace{-1.5mm} &
\includegraphics[width=0.186\textwidth]{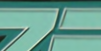} \hspace{-1.5mm} &
\includegraphics[width=0.186\textwidth]{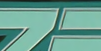} \hspace{-1.5mm} &
\includegraphics[width=0.186\textwidth]{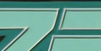} \hspace{-1.5mm}  
\\ 
Bicubic \hspace{-1.5mm} &
LatticeNet~\cite{luo2020latticenet}  \hspace{-1.5mm} &
\textcolor{black}{\textbf{HiT-SIR} (Ours)}  \hspace{-1.5mm} &
\textcolor{black}{\textbf{HiT-SRF} (Ours)} \hspace{-1.5mm}
\\
\end{tabular}
\end{adjustbox}
\\
% % one row
\hspace{-0.2cm}
\begin{adjustbox}{valign=t}
\begin{tabular}{c}
\includegraphics[width=0.265\textwidth]{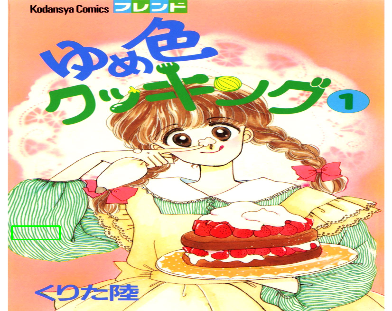}
\\
YumeiroCooking 
\end{tabular}
\end{adjustbox}
\hspace{-0.23cm}
\begin{adjustbox}{valign=t}
\begin{tabular}{ccccc}
\includegraphics[width=0.186\textwidth]{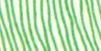} \hspace{-1.5mm} &
\includegraphics[width=0.186\textwidth]{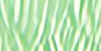} \hspace{-1.5mm} &
\includegraphics[width=0.186\textwidth]{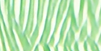} \hspace{-1.5mm} &
\includegraphics[width=0.186\textwidth]{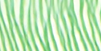} \hspace{-1.5mm} 
\\
HR \hspace{-1.5mm} &
IMDN~\cite{hui2019imdn} \hspace{-1.5mm} &
SwinIR-Light~\cite{liang2021swinir} \hspace{-1.5mm} &
SRFormer-Light~\cite{Zhou_2023srformer} \hspace{-1.5mm} 
\\
\includegraphics[width=0.186\textwidth]{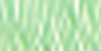} \hspace{-1.5mm} &
\includegraphics[width=0.186\textwidth]{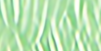} \hspace{-1.5mm} &
\includegraphics[width=0.186\textwidth]{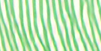} \hspace{-1.5mm} &
\includegraphics[width=0.186\textwidth]{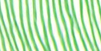} \hspace{-1.5mm}  
\\ 
Bicubic \hspace{-1.5mm} &
LatticeNet~\cite{luo2020latticenet}  \hspace{-1.5mm} &
\textcolor{black}{\textbf{HiT-SIR} (Ours)}  \hspace{-1.5mm} &
\textcolor{black}{\textbf{HiT-SRF} (Ours)} \hspace{-1.5mm}
\\
\end{tabular}
\end{adjustbox}
\\
% % one row ----------------------
\hspace{-0.2cm}
\begin{adjustbox}{valign=t}
\begin{tabular}{c}
\includegraphics[width=0.265\textwidth]{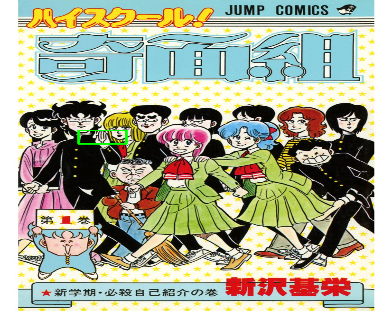}
\\
HighschoolKimengumi\_vol01 
\end{tabular}
\end{adjustbox}
\hspace{-0.23cm}
\begin{adjustbox}{valign=t}
\begin{tabular}{ccccc}
\includegraphics[width=0.186\textwidth]{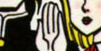} \hspace{-1.5mm} &
\includegraphics[width=0.186\textwidth]{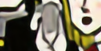} \hspace{-1.5mm} &
\includegraphics[width=0.186\textwidth]{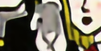} \hspace{-1.5mm} &
\includegraphics[width=0.186\textwidth]{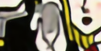} \hspace{-1.5mm} 
\\
HR \hspace{-1.5mm} &
IMDN~\cite{hui2019imdn} \hspace{-1.5mm} &
SwinIR-Light~\cite{liang2021swinir} \hspace{-1.5mm} &
SRFormer-Light~\cite{Zhou_2023srformer} \hspace{-1.5mm} 
\\
\includegraphics[width=0.186\textwidth]{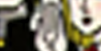} \hspace{-1.5mm} &
\includegraphics[width=0.186\textwidth]{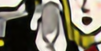} \hspace{-1.5mm} &
\includegraphics[width=0.186\textwidth]{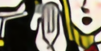} \hspace{-1.5mm} &
\includegraphics[width=0.186\textwidth]{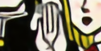} \hspace{-1.5mm}  
\\ 
Bicubic \hspace{-1.5mm} &
LatticeNet~\cite{luo2020latticenet}  \hspace{-1.5mm} &
\textcolor{black}{\textbf{HiT-SIR} (Ours)}  \hspace{-1.5mm} &
\textcolor{black}{\textbf{HiT-SRF} (Ours)} \hspace{-1.5mm}
\\
\end{tabular}
\end{adjustbox}
\\
% % one row ----------------------
\hspace{-0.2cm}
\begin{adjustbox}{valign=t}
\begin{tabular}{c}
\includegraphics[width=0.265\textwidth]{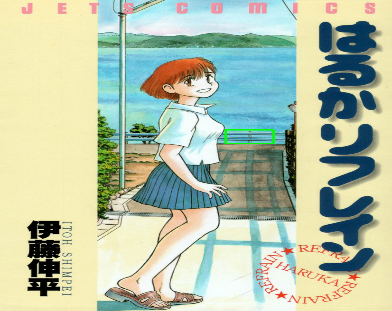}
\\
HarukaRefrain 
\end{tabular}
\end{adjustbox}
\hspace{-0.23cm}
\begin{adjustbox}{valign=t}
\begin{tabular}{ccccc}
\includegraphics[width=0.186\textwidth]{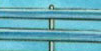} \hspace{-1.5mm} &
\includegraphics[width=0.186\textwidth]{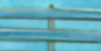} \hspace{-1.5mm} &
\includegraphics[width=0.186\textwidth]{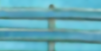} \hspace{-1.5mm} &
\includegraphics[width=0.186\textwidth]{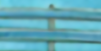} \hspace{-1.5mm} 
\\
HR \hspace{-1.5mm} &
IMDN~\cite{hui2019imdn} \hspace{-1.5mm} &
SwinIR-Light~\cite{liang2021swinir} \hspace{-1.5mm} &
SRFormer-Light~\cite{Zhou_2023srformer} \hspace{-1.5mm} 
\\
\includegraphics[width=0.186\textwidth]{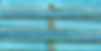} \hspace{-1.5mm} &
\includegraphics[width=0.186\textwidth]{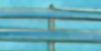} \hspace{-1.5mm} &
\includegraphics[width=0.186\textwidth]{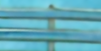} \hspace{-1.5mm} &
\includegraphics[width=0.186\textwidth]{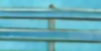} \hspace{-1.5mm}  
\\ 
Bicubic \hspace{-1.5mm} &
LatticeNet~\cite{luo2020latticenet}  \hspace{-1.5mm} &
\textcolor{black}{\textbf{HiT-SIR} (Ours)}  \hspace{-1.5mm} &
\textcolor{black}{\textbf{HiT-SRF} (Ours)} \hspace{-1.5mm}
\\
\end{tabular}
\end{adjustbox}
\\
% % one row ----------------------
\hspace{-0.2cm}
\begin{adjustbox}{valign=t}
\begin{tabular}{c}
\includegraphics[width=0.265\textwidth]{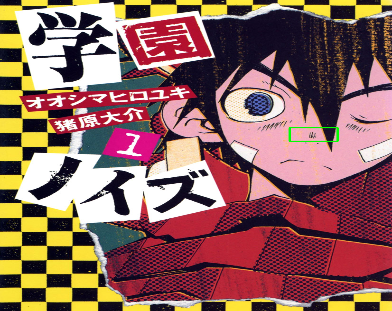}
\\
GakuenNoise 
\end{tabular}
\end{adjustbox}
\hspace{-0.23cm}
\begin{adjustbox}{valign=t}
\begin{tabular}{ccccc}
\includegraphics[width=0.186\textwidth]{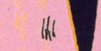} \hspace{-1.5mm} &
\includegraphics[width=0.186\textwidth]{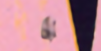} \hspace{-1.5mm} &
\includegraphics[width=0.186\textwidth]{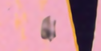} \hspace{-1.5mm} &
\includegraphics[width=0.186\textwidth]{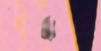} \hspace{-1.5mm} 
\\
HR \hspace{-1.5mm} &
IMDN~\cite{hui2019imdn} \hspace{-1.5mm} &
SwinIR-Light~\cite{liang2021swinir} \hspace{-1.5mm} &
SRFormer-Light~\cite{Zhou_2023srformer} \hspace{-1.5mm} 
\\
\includegraphics[width=0.186\textwidth]{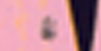} \hspace{-1.5mm} &
\includegraphics[width=0.186\textwidth]{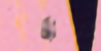} \hspace{-1.5mm} &
\includegraphics[width=0.186\textwidth]{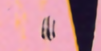} \hspace{-1.5mm} &
\includegraphics[width=0.186\textwidth]{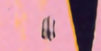} \hspace{-1.5mm}  
\\ 
Bicubic \hspace{-1.5mm} &
LatticeNet~\cite{luo2020latticenet}  \hspace{-1.5mm} &
\textcolor{black}{\textbf{HiT-SIR} (Ours)}  \hspace{-1.5mm} &
\textcolor{black}{\textbf{HiT-SRF} (Ours)} \hspace{-1.5mm}
\\
\end{tabular}
\end{adjustbox}
\\
% % one row ----------------------
\hspace{-0.2cm}
\begin{adjustbox}{valign=t}
\begin{tabular}{c}
\includegraphics[width=0.265\textwidth]{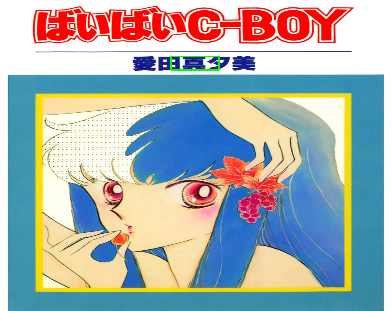}
\\
ByebyeC-BOY 
\end{tabular}
\end{adjustbox}
\hspace{-0.23cm}
\begin{adjustbox}{valign=t}
\begin{tabular}{ccccc}
\includegraphics[width=0.186\textwidth]{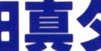} \hspace{-1.5mm} &
\includegraphics[width=0.186\textwidth]{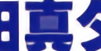} \hspace{-1.5mm} &
\includegraphics[width=0.186\textwidth]{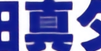} \hspace{-1.5mm} &
\includegraphics[width=0.186\textwidth]{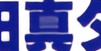} \hspace{-1.5mm} 
\\
HR \hspace{-1.5mm} &
IMDN~\cite{hui2019imdn} \hspace{-1.5mm} &
SwinIR-Light~\cite{liang2021swinir} \hspace{-1.5mm} &
SRFormer-Light~\cite{Zhou_2023srformer} \hspace{-1.5mm} 
\\
\includegraphics[width=0.186\textwidth]{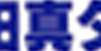} \hspace{-1.5mm} &
\includegraphics[width=0.186\textwidth]{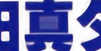} \hspace{-1.5mm} &
\includegraphics[width=0.186\textwidth]{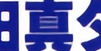} \hspace{-1.5mm} &
\includegraphics[width=0.186\textwidth]{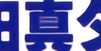} \hspace{-1.5mm}  
\\ 
Bicubic \hspace{-1.5mm} &
LatticeNet~\cite{luo2020latticenet}  \hspace{-1.5mm} &
\textcolor{black}{\textbf{HiT-SIR} (Ours)}  \hspace{-1.5mm} &
\textcolor{black}{\textbf{HiT-SRF} (Ours)} \hspace{-1.5mm}
\\
\end{tabular}
\end{adjustbox}
\\

\end{tabular} }
% \vspace{-3mm}
\caption{{Qualitative comparisons for image SR on Manga109 ($\times 4$).}}
\label{fig:qualires-m109}
% \vspace{-2em}
\end{figure*}
