# Supplementary material for: HiT-SR: Hierarchical Transformer for Efficient Image Super-Resolution
Source: arXiv:2407.05878 source file (2024-07-08)
Supplement: Supplementary file 2 [file fig-DPE.tex]

% \begin{figure}[!t]
\begin{wrapfigure}{r}{0.5\linewidth}
    \centering
    % \vspace{-4mm}
    \includegraphics[width=0.9\linewidth]{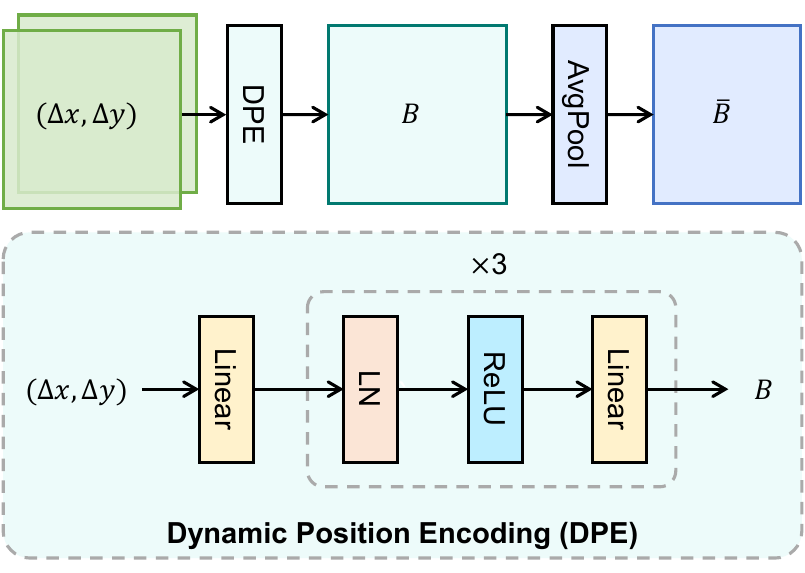}
    % \vspace{-0.5em}
    \caption{Position encoding in HiT-SR. Following \cite{wang2023crossformer++}, a dynamic position encoding (DPE) network composed of linear layers, layer normalization (LN), and ReLU activations is first employed to convert coordinate distance matrices, \ie, $\Delta x$ and $\Delta y$, to position bias $B$. An average pooling layer is then applied on $B$ to model spatial relations between queries $Q$ and projected values $V_{\downarrow}$. }
    \label{fig:DPE}
    % \vspace{-1em}
\end{wrapfigure}
