# Supplementary material for: HiT-SR: Hierarchical Transformer for Efficient Image Super-Resolution
Source: arXiv:2407.05878 source file (2024-07-08)
Supplement: Supplementary file 3 [file fig-LAM.tex]

\begin{figure*}[t]
\centering
\begin{subfigure}{0.19\textwidth}
    \includegraphics[width=\linewidth]{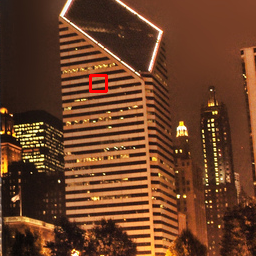}
\\
\includegraphics[width=\linewidth]{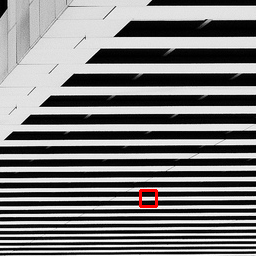}
\\
\includegraphics[width=\linewidth]{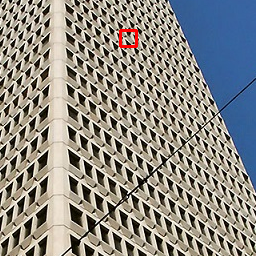}
\\
\includegraphics[width=\linewidth]{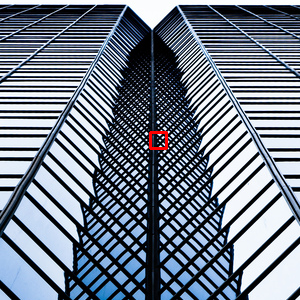}
\\
\includegraphics[width=\linewidth]{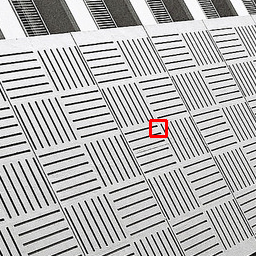}
    \caption*{Target Region}
\end{subfigure}
%% new coloumn
\begin{subfigure}{0.19\textwidth}
\includegraphics[width=\linewidth]{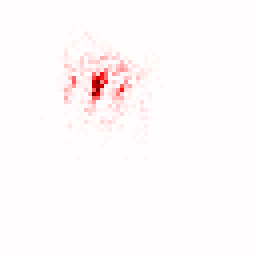}
\\
\includegraphics[width=\linewidth]{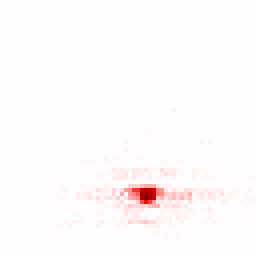}
\\
\includegraphics[width=\linewidth]{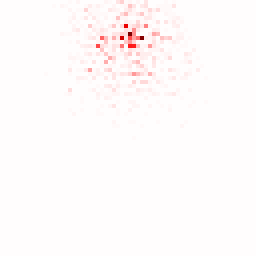}
\\
\includegraphics[width=\linewidth]{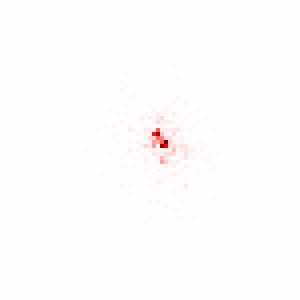}
\\
\includegraphics[width=\linewidth]{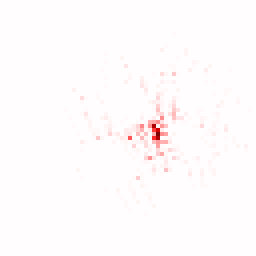}
    \caption*{LAM (SwinIR-Light)}
\end{subfigure}
%% new coloumn
\begin{subfigure}{0.19\textwidth}
    \includegraphics[width=\linewidth]{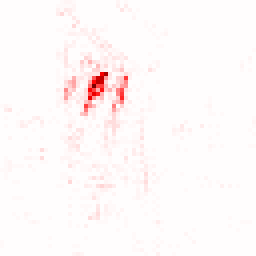}
\\
\includegraphics[width=\linewidth]{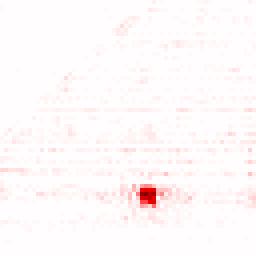}
\\
\includegraphics[width=\linewidth]{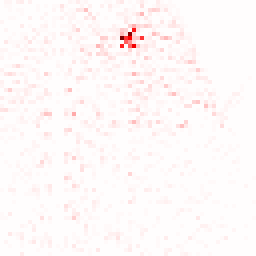}
\\
\includegraphics[width=\linewidth]{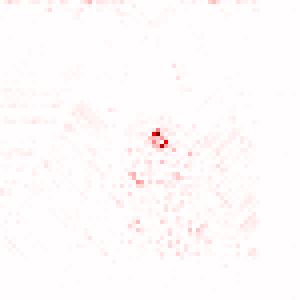}
\\
\includegraphics[width=\linewidth]{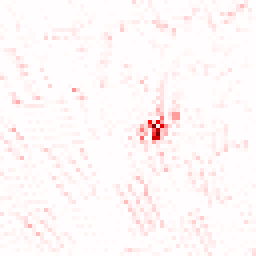}
    \caption*{LAM (HiT-SIR)}
\end{subfigure}
%% new coloumn
\begin{subfigure}{0.19\textwidth}
    \includegraphics[width=\linewidth]{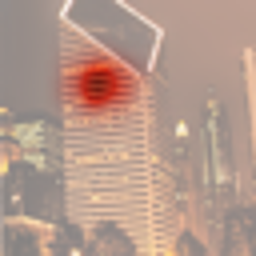}
\\
\includegraphics[width=\linewidth]{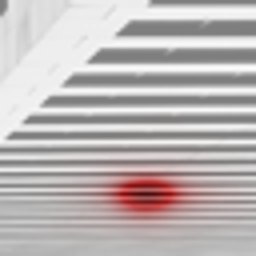}
\\
\includegraphics[width=\linewidth]{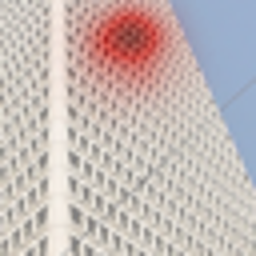}
\\
\includegraphics[width=\linewidth]{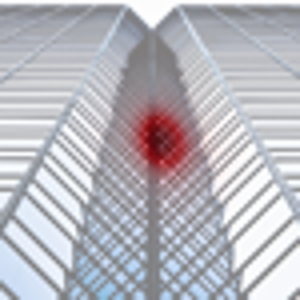}
\\
\includegraphics[width=\linewidth]{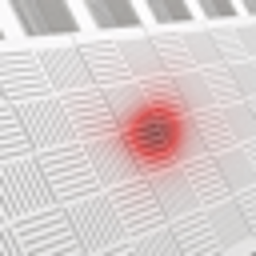}
    \caption*{Inform. Area (SwinIR-Light)}
\end{subfigure}
%% new coloumn
\begin{subfigure}{0.19\textwidth}
    \includegraphics[width=\linewidth]{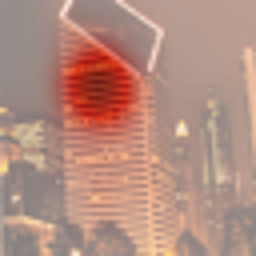}
\\
\includegraphics[width=\linewidth]{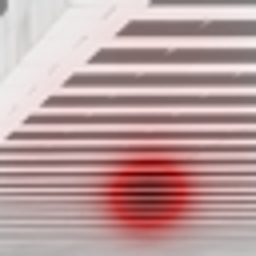}
\\
\includegraphics[width=\linewidth]{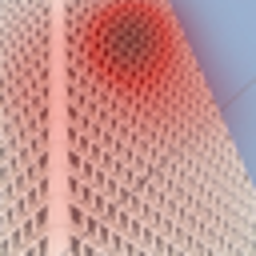}
\\
\includegraphics[width=\linewidth]{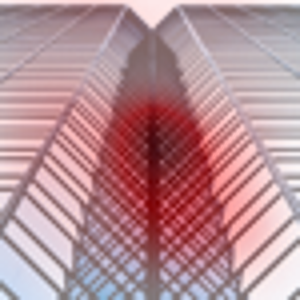}
\\
\includegraphics[width=\linewidth]{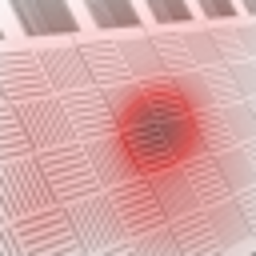}
    \caption*{Inform. Area (HiT-SIR)}
\end{subfigure}
	\caption{Comparisons between SwinIR-Light and our HiT-SIR, where local attribution maps (LAM) and informative areas are illustrated. }
	\label{fig:lam}
\end{figure*}
