# Supplementary material for: HiT-SR: Hierarchical Transformer for Efficient Image Super-Resolution
Source: arXiv:2407.05878 source file (2024-07-08)
Supplement: Supplementary file 4 [file fig-channel-adjusting.tex]

\def\scale{0.48}
\begin{figure}[t]
% \vspace{-1em}
    \centering
\begin{subfigure}{0.9\linewidth}
\centering
%% for performance ==========================
% for params
       \begin{tikzpicture}[scale=\scale]
		\begin{axis}
			[
             height=0.6\linewidth,
             width=\linewidth,
             ymin=38.9, ymax=39.26,
              ylabel={PSNR (dB)},
              xlabel={FLOPs (G)},
              line width=1.2pt,
			 axis y line=left,
			 axis x line=bottom,
              every axis/.append style={font=\large},
              grid,
              nodes near coords,
    point meta=explicit symbolic,
              % legend pos=south east,
              legend style={at={(0.2,1.2)},anchor=north,legend columns=-1},
    grid style={color=white, line width=0.5pt},
              axis background/.style={fill=gray!10}, % 设置背景颜色
			 enlarge x limits=0.1, ] 
			\addplot[only marks, mark size=4pt,mark=triangle,color=blue] coordinates {
                  (194.1, 38.98) [\#6*]
                };
                % \addlegendentry{\#6*}
                \addplot[only marks, mark size=4pt,mark=square,color=blue, every node near coord/.append style={anchor=east}] coordinates {
                  (189.1, 38.92) [\#7*]
                };
                % \addlegendentry{\#7*}
                \addplot[only marks, mark size=4pt,mark=o,color=blue] coordinates {
                  (189.1, 38.95) [\#11*]
                };
                % \addlegendentry{\#11*}
                \addplot[only marks, mark size=4pt,mark=diamond,color=blue] coordinates {
                  (179.7, 39.15) [\#12*]
                };
                % \addlegendentry{\#12*}
                % %
                \addplot[only marks, mark size=4pt,mark=star,color=black] coordinates {
                  (209.9, 39.21) [\textbf{Ours}]
                };
                % \addlegendentry{\textbf{Ours}}
                % %
                \addplot[only marks, mark size=4pt,mark=triangle,color=red] coordinates {
                  (214.9, 38.99) [\#6]
                };
                % \addlegendentry{\#6}
                \addplot[only marks, mark size=4pt,mark=square,color=red] coordinates {
                  (212.3, 38.95) [\#7]
                };
                % \addlegendentry{\#7}
                \addplot[only marks, mark size=4pt,mark=o,color=red] coordinates {
                  (222.1, 39.04) [\#11]
                };
                % \addlegendentry{\#11}
                \addplot[only marks, mark size=4pt,mark=diamond,color=red] coordinates {
                  (217.2, 39.18) [\#12]
                };
                % \addlegendentry{\#12}
		\end{axis} 
	\end{tikzpicture} 
 %% PSNR - Param
 \begin{tikzpicture}[scale=\scale]
		\begin{axis}
			[
             height=0.6\linewidth,
             width=\linewidth,
             ymin=38.9, ymax=39.26,
              ylabel={PSNR (dB)},
              xlabel={\#Para. (K)},
              line width=1.2pt,
			 axis y line=left,
			 axis x line=bottom,
              every axis/.append style={font=\large},
              grid,
              nodes near coords,
    point meta=explicit symbolic,
              % legend pos=south east,
              legend style={at={(0.2,1.2)},anchor=north,legend columns=-1},
    grid style={color=white, line width=0.5pt},
              axis background/.style={fill=gray!10}, % 设置背景颜色
			 enlarge x limits=0.1, ] 
			\addplot[only marks, mark size=4pt,mark=triangle,color=blue] coordinates {
                  (704, 38.98) [\#6*]
                };
                % \addlegendentry{\#6*}
                \addplot[only marks, mark size=4pt,mark=square,color=blue, every node near coord/.append style={anchor=south}] coordinates {
                  (684, 38.92) [\#7*]
                };
                % \addlegendentry{\#7*}
                \addplot[only marks, mark size=4pt,mark=o,color=blue] coordinates {
                  (729, 38.95) [\#11*]
                };
                % \addlegendentry{\#11*}
                \addplot[only marks, mark size=4pt,mark=diamond,color=blue] coordinates {
                  (727, 39.15) [\#12*]
                };
                % \addlegendentry{\#12*}
                % %
                \addplot[only marks, mark size=4pt,mark=star,color=black] coordinates {
                  (772, 39.21) [\textbf{Ours}]
                };
                % \addlegendentry{\textbf{Ours}}
                % %
                \addplot[only marks, mark size=4pt,mark=triangle,color=red] coordinates {
                  (792, 38.99) [\#6]
                };
                % \addlegendentry{\#6}
                \addplot[only marks, mark size=4pt,mark=square,color=red] coordinates {
                  (781, 38.95) [\#7]
                };
                % \addlegendentry{\#7}
                \addplot[only marks, mark size=4pt,mark=o,color=red] coordinates {
                  (819, 39.04) [\#11]
                };
                % \addlegendentry{\#11}
                \addplot[only marks, mark size=4pt,mark=diamond,color=red] coordinates {
                  (816, 39.18) [\#12]
                };
                % \addlegendentry{\#12}
		\end{axis} 
	\end{tikzpicture} 
\end{subfigure}
    % \vspace{-1em}
    \caption{PSNR with respect to FLOPs and \#Para. of the ablated models \#6, \#7, \#11, and \#12 in Tab. 4 of our main paper. * means models without channel adjusting. }
    \label{fig:channel-adjusting}
    % \vspace{-1em}
\end{figure}
