# Supplementary material for: HiT-SR: Hierarchical Transformer for Efficient Image Super-Resolution
Source: arXiv:2407.05878 source file (2024-07-08)
Supplement: Supplementary file 6 [file fig-splinear.tex]

% \begin{figure}[!ht]
\begin{wrapfigure}{r}{0.5\linewidth}
    \centering
    % \vspace{-2mm}
    \includegraphics[width=\linewidth]{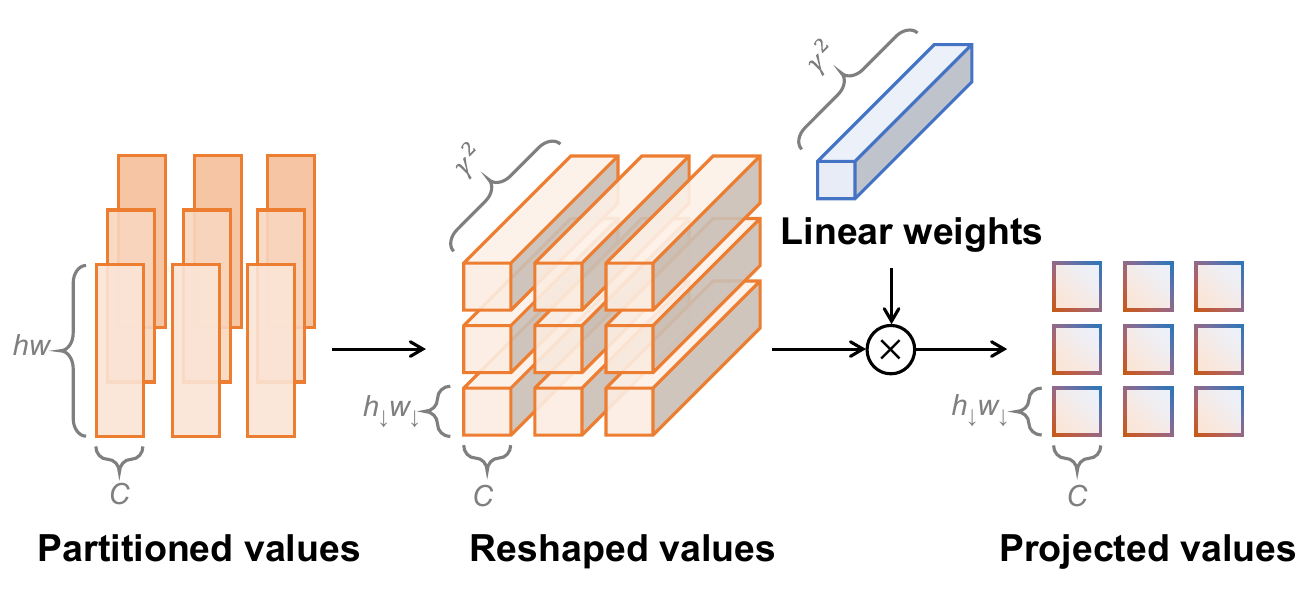}
    % \vspace{-0.5em}
    \caption{Pipeline of spatial linear projection. In this example, the value is partitioned to 9 windows. Each partitioned value $V\in\mathbb{R}^{h w\times C}$ is first reshaped to the $\mathbb{R}^{h_\downarrow w_\downarrow \times C\times \gamma^2}$ space. Then a weight-sharing linear layer is applied to summarize spatial information for each window, \ie, $\mathbb{R}^{\gamma^2}\rightarrow\mathbb{R}^{1}$, producing the projected values $V_{\downarrow}\in\mathbb{R}^{h_\downarrow w_\downarrow \times C}$.  }
    \label{fig:splinear}
    % \vspace{-1em}
\end{wrapfigure}
% \end{figure}
