# Supplementary material for: HiT-SR: Hierarchical Transformer for Efficient Image Super-Resolution
Source: arXiv:2407.05878 source file (2024-07-08)
Supplement: Supplementary file 7 [file tab-ablation.tex]

\begin{table}[t]
\scriptsize
\caption{Additional ablation studies. We train all models on the DIV2K dataset for 300K iterations, and test them on the Manga109 ($\times 2$) dataset. The ablations about correlation \vs attention, window diversity, max window size, base window size, and more window strategies correspond to experiments \#1-2, \#3-6, \#7-9, \#10-13, and \#14-16. Win. indicates the assigned window sizes for a transformer block, and the best SR results are colored \textcolor{red}{red}.}
\label{table:supp-ablation}
\begin{center}
\setlength\tabcolsep{5pt}

\begin{tabular}{c|c|cc|cc}
\toprule[0.15em]
\rowcolor{color3}
ID   & Strategies                       & \#Para. & FLOPs & PSNR & SSIM \\ 
\midrule[0.15em]
\#1  & {QV correlation}  & 772K         & 209.9G      & \textcolor{red}{39.21}     & \textcolor{red}{0.9780}    \\
\#2  & QKV attention       & 826K         &  222.6G     & \textcolor{black}{39.09}     &  \textcolor{black}{0.9778}    \\
\midrule
\#3  & Win.={[}8,8,8,8,8,8{]}   &  772K      & 208.6G    & 38.88    &  0.9775    \\
\#4  & Win.={[}8,8,8,16,16,16{]}   &  772K      & 209.5G    & 39.01     &  0.9774    \\
\#5  & Win.={[}8,8,16,16,32,32{]}                         &  772K       &  211.1G     &  \textcolor{black}{39.10}    &  \textcolor{black}{0.9779}   \\
\#6  & {Win.={[}4,8,16,32,48,64{]}} & 772K         & 209.9G      & \textcolor{red}{39.21}     & \textcolor{red}{0.9780}     \\
\midrule
\#7  & Win.={[}4,6,8,16,24,32{]}     &  772K      &  205.9G     &  39.15    & \textcolor{black}{0.9780}     \\
\#8  & {Win.={[}4,8,16,32,48,64{]}} & 772K         & 209.9G      & \textcolor{black}{39.21}     & \textcolor{black}{0.9780}     \\
\#9  & Win.={[}4,8,16,32,64,96{]}  &   773K      &  209.9G    &  \textcolor{red}{39.23}    &  \textcolor{red}{0.9782}  \\
\midrule
\#10 & [$h_B,w_B$]=[2,2]        &  779K   & 191.7G     &  39.19    & \textcolor{black}{0.9780}     \\
\#11 & [$h_B,w_B$]=[4,4]    &  774K  &  195.9G   &  \textcolor{red}{39.22} &  \textcolor{red}{0.9781}       \\
\#12 & {[$h_B,w_B$]=[8,8]}                         &  772K        & 209.9G      &  \textcolor{black}{39.21}    &  \textcolor{black}{0.9780}  \\
\#13 & [$h_B,w_B$]=[16,16]       &   772K     & 255.3G     &  39.18 & \textcolor{black}{0.9780}   \\
\midrule
\#14  & Win.={[}4,16,64,64,16,4{]}     &  772K      &  205.8G     &  39.18    & \textcolor{black}{0.9778}     \\
\#15  & {Win.={[}64,16,4,4,16,64{]}} & 772K         & 205.8G      & \textcolor{black}{39.13}     & \textcolor{black}{0.9778}     \\
\#16  & Win.={[}8,4,32,16,64,48{]}  &   772K      &  209.9G    &  \textcolor{red}{39.20}    &  \textcolor{red}{0.9781}  \\
\bottomrule[0.15em]
\end{tabular}

\end{center}
% \vspace{-8mm}
\vspace{-0.5em}
\end{table}
